# Supplementary material for: Testing Quantum Dissipation Theory with Electron Diffraction
Source: arXiv:2201.08525 source file (2022-01-21)
Supplement: Supplementary file 1 [file appendix.tex]

\section{info}
% model details
%Zurek
In Anglin and Zurek's original model~\cite{Anglin97}, the Caldeira-Leggett master equation gives the evolution of the free electron's density matrix affected by the quantum Brownian motion. The model shows that the resistivity sets the decoherence rate and the energy dissipation rate. It was stated that the model should work for resistivity in the $10^{-8} \Omega$ cm to $10^{8} \Omega$ cm range. The decoherence time of the electron flying above the wall (semiconductor) is given by ~\cite{Anglin97,Beierle18}, 
 \begin{equation}
 \tau_{\mathrm{dec}}^{\text {Zurek }}=\frac{4 h^{2}}{\pi e^{2} k_{\mathrm{B}} T \rho} \frac{z^{3}}{(\Delta x)^{2}},
 \label{eqn:Zurek}
 \end{equation}
where $h$ is the Plank constant, $k_{\mathrm{B}}$ is the Boltzmann constant, $T=300$ $\mathrm{K}$ is the temperature, $\rho$ is the resistivity of the sample, $z$ is the electron height above the surface, $\Delta x$ is the path distance. However, in our experiment, we should add two correction factors (see Appendix D for details). The first factor is needed as the image charge patches under the electron path have overlap which reduces their capability to distinguish flying electron superposition states by a factor of $(z/\Delta x)^{2}$[Private communication with Zurek]. 
The second factor is needed as the GaAs surface location is placed in the transition region between the near- and far-field electron diffraction pattern. This means that the superposition of paths from the slits to the detection do not separate entirely. This correction shares the same idea that the overlap of two entangled states reduce the environmental induced decoherence rate compared to rate of two well separated initial states. Here we estimated it to be a factor of $(\omega/\Delta x)^{2}$ where $\omega$ is the average width of a single slit beam above the surface.

% Howie
The general differential form of the single event probability $P$ is  
\begin{equation}
\frac{d^{2} P\left(y, \omega, q_{x}\right)}{d \omega d q_{x}}=\frac{e^{2} L}{2 \pi^{2} \varepsilon_{0} \hbar v^{2}} \operatorname{Im}\{\lambda_{e}\} \exp \left[-2 \nu_{0} z\right],
\label{eqn:event probability} 
\end{equation}
where $\lambda_{e}$ is the retarded loss function (see Supplementary Materials). Previously, it was given in different forms [Howie, Forstamann]. First, Eq.~(\ref{eqn:event probability}) is integrated over the plasmon frequency $\omega$. The upper bound of the plasmon frequency can be estimated from Eq.~(\ref{eqn:event probability}) which falls off quickly so that it doesn't contribute to the integral at large frequency [Howie2011, kerker, beierle]. To decohere, the flying electron must get a momentum recoil larger than its momentum spread and thus "sufficient to distinguish between the two interference paths"~\cite{Howie11}. Relating this to our the experiment this can be rephrased as follows. The transverse coherence length sets the momentum spread of the motional quantum state according to Heisenberg's uncertainty principle. A momentum recoil larger than this momentum spread can thus distinguish the quantum state and cause decoherence.  This implies that one should integrate the wave vector in the range of $q_{x}>\alpha \Delta x$, where $\alpha$ depends on the specific wavefunction and is of the order of one. The value used in [Howie2011] here is $1/8$ to get agreement with the experiment by Hasselbach [Hasselbach] (note that there was a typographical error in~\cite{Howie11}; $\alpha$ was mistakenly written as two [howie11Private Communication]). The relative dielectric function, $\varepsilon=1+i\sigma/\varepsilon_{0}\omega$ given by the Drude model, is used in these papers. Not previously used for the calculation of decoherence rates, is that Eq.~(\ref{eqn:event probability}) needs to be multiplied with the usual Boltzmann thermal correction factor $\operatorname{coth}\left(\frac{\hbar \omega}{2 k T}\right)$[private communication, Howie2019]. Even if Howie's model also predict energy loss it is not associated with the decoherence as an example of the Caldeira-Leggett equation.  

% Scheel
The theory is modified to include the finite temperature correction by inclusion of the Bose-Einstein distribution: 
\begin{equation}
\bar{n}_{\mathrm{th}}(\omega)=\left[e^{\hbar \omega /\left(k_{B} T\right)}-1\right]^{-1}.
\end{equation}
The interference visibility is given by $e^{-\Gamma[c]}$, where 
\begin{equation}
\begin{array}{lll}
\Gamma[c]&=-\frac{q^{2} t}{\epsilon_{0} \hbar(2 \pi)^{2}} \int_{-\infty}^{\infty} \int_{-\infty}^{\infty} \mathrm{d} k_{x} \mathrm{~d} k_{y}\left(1-\cos \left(k_{x} L\right)\right)&\\
&\times \left(2 \bar{n}_{\mathrm{th}}\left(\left|k_{y} v\right|\right)+1\right)
\times \frac{\mathrm{e}^{-2 k_{\|} z \gamma\left(k_{x}, k_{y}\right)}}{2 k_{\|} \gamma\left(k_{x}, k_{y}\right)}&\\
&\times \operatorname{Im}\left(r_{\mathrm{p}}\left(k_{\|},\left|k_{y} v\right|\right) \gamma^{2}+r_{\mathrm{s}}\left(k_{\|},\left|k_{y} v\right|\right) \frac{v^{2}}{c^{2}} \frac{k_{x}^{2}}{k_{\|}^{2}}\right),&
\end{array}
\end{equation}
where the reflection coefficients $r_{\mathrm{s}}$ and $r_{\mathrm{p}}$ depend on the resistivity (Supplementary Materials).

% supplimentary info

\section{Decoherence theory}
In Zurek's theory, the relation between decoherence time and relaxation time is given by 
\begin{equation}
\tau_{\mathrm{dec}}^{\mathrm{Zurek}}=\left(\frac{\lambda_{\mathrm{th}}}{\Delta x}\right)^{2} \tau_{\mathrm{relax}},
\end{equation}
where $\Delta x$ is the coherence length for our experiment and $\lambda_{\mathrm{th}}=\hbar / \sqrt{m k_{b} T}$ is the thermal de Broglie wavelength of the electron in the room temperature (300 K). This equation derived from Caldeira-Leggett master equation describes the decoherence caused by energy loss when the electron passing above a resistive surface. The definition of relaxation time is $\tau_{\text {relax }} \equiv v /\left|\frac{d v}{d t}\right|$ according to Zeh[]. The energy loss due to Ohmic dissipation used in Zurek's model comes from Boyer's theory[]:
\begin{equation}\label{elossrate}
P=\frac{e^{2} \rho v^{2}}{16 \pi z^{3}}.
\end{equation}
By definition,
\begin{equation}
P=m v \dot{v}=\frac{m v^{2}}{\tau_{\text {relax }}} \rightarrow \tau_{\text {relax}}=\frac{m v^{2}}{P},
\end{equation}
in our experiment, the decoherence rate is calculated by
\begin{equation}
R^{Zurek}_{dec}=\int{\frac{dt}{\tau_{dec}^{Zurek}}}=\left(\frac{\Delta x}{\lambda_{\mathrm{th}}}\right)^{2} \frac{\Delta E}{mv^{2}},
\end{equation}
where $\Delta E$ is the energy loss during the interaction.

In Howie's theory, the general form of event probability is given in Eq.~\ref{eqn:event probability} but several different form of retarded loss function is given in the literature. In this paper, we used the form:

\begin{equation}
\lambda_{e}=-\frac{2}{\nu+\nu_{0} \varepsilon}+\frac{2 \beta^{2}}{\nu+\nu_{0}},
\end{equation}
where $\beta=v/c$, $\nu_{0}^{2}=\left[q_{x}^{2}+(\omega / v)^{2}-(\omega / c)^{2}\right]$, $\nu^{2}=\left[q_{x}^{2}+(\omega / v)^{2}-\varepsilon(\omega)(\omega / c)^{2}\right]$. The dielectric function, we use $\varepsilon(\omega) \approx 1+i \sigma(T) / \varepsilon_{0} \omega$m where $\sigma$ is the conductivity of the surface.

\begin{equation}
P^{\text {Howie }}=\left(\frac{e^{2} L \omega_{m}^{2}}{4 \pi^{2} \hbar \sigma v^{2}}\right) \int_{z / 4 \Delta x}^{\infty} \frac{\exp (-s)}{s} \mathrm{~d} s,
\end{equation}

where $L$ is the path length which is approximately the sample length, $\omega_{m}$ is the cut-off frequency for a semiconductor, $\sigma=1/\rho$ is the conductivity. A full transition from quantum to classical is thus predicted.
